# Supplementary material for: A Thorough Investigation of Content-Defined Chunking Algorithms for Data Deduplication
Source: arXiv:2409.06066 source file (2024-09-28)
Supplement: Supplementary file 1 [file ae_stochastics.tex]

\begin{definition}
	In AE, $i+h$ marks a cut-point if it is the first position for which $B_i\geq\max\{B_j\}_{j=i+1}^{i+h}$.
\end{definition}

In order for any byte $B_i$ at position $i$ to become subject to the matching condition,
all previous bytes $B_{j<i}$ must have failed the matching condition $B_j\geq\max\{B_k\}_{k=j+1}^{j+h}$.
However, these are not independent events.
The event $B_{i-1}<\max\{B_{j}\}_{j=i}^{i+h-1}$ influences the expectation of $B_{i},\ldots,B_{i+h}$, and therefore affects the probability $B_i<\max\{B_j\}_{j=i+1}^{i+h}$.
So does every previous condition back to $B_{i-h-1}<\max\{B_j\}_{j=i-h}^i$ as it still influences the expected value of $B_i$.
This leads to a \textbf{chain of recursive conditional probabilities} that we express as:

\begin{equation}
\begin{split}
    \mathrm{P}(i+h\text{ marks cut-point})= \mathrm{P}(B_i\geq \max\{B_j\}_{j=i+1}^{i+h}\mid B_{i-1}<\max\{B_j\}_{j=i}^{i+h-1}\land\ldots\land
    B_{i-h-1}<\max\{B_j\}_{j=i-h}^{i})\cdot\\\ldots\cdot\mathrm{P}(B_2<\max\{B_j\}_{j=3}^{h+2}\mid B_1<\max\{B_j\}_{j=2}^{h+1})\cdot\mathrm{P}(B_1<\max\{B_j\}_{j=2}^{h+1})
\end{split}
\end{equation}

For the purpose of readability, we introduce the abbreviation $M_h := \max\{B_i\}_{i=1}^h$ to denote the maximum value among $h$ bytes. 
As we are assuming uniformly distributed random data, and bytes are discrete variables in $[0,255]$,
the probability for any byte $X$ to take any value $0\leq x\leq 255$ is $P(X=x)=1/256$.
Furthermore, $P(X<x)=\frac{x}{256}$, $P(X\geq x)=\frac{256-x}{256}$, $P(X<Y)=\frac{1}{2}$, and $P(X\leq Y)=\frac{257}{512}$.

\begin{lemma}
	The cumulative distribution function $F_M(m)=\mathrm{P}(\max\{B_i\}_{i=1}^h\leq m)$ follows
	\begin{equation}
		F_{M_h}(m)=\mathrm{P}(B_1\leq m\land\ldots B_h\leq m)=\left(\frac{m+1}{256}\right)^h\quad\text{for }0\leq m\leq 255
	\end{equation}
	
	and can be used to express the probability mass function of $M_h$:

	\begin{equation}
    	\mathrm{P}(M_h = m) = F_{M_h}(m)-F_{M_h}(m-1)=\left(\frac{m+1}{256}\right)^h-\left(\frac{m}{256}\right)^h\quad\text{for }0\leq m\leq 255
    \label{eq:ae_mh_m}
	\end{equation}

	Further, a lower bound $x$ changes this distribution to

	\begin{equation}
    	\mathrm{P}(M_h=m\mid M_h\geq x) = \left(\frac{m-x+1}{256-x}\right)^h-\left(\frac{m-x}{256-x}\right)^h\quad \text{for } 0 \leq m \leq 255 \quad \text{and} \quad 0 \leq x \leq 255.
	\label{eq:eight}
	\end{equation}
\end{lemma}

\begin{figure}[h]
    \centering
    \input{figures/ae_pmf.tex}
    \caption{Probability mass function for $M_h$. Note, $m$ is discrete; line plots were chosen for readability. As $h$ increases, the expected value for $M_h$ converges to 255.}
    \label{fig:ae_pmf}
\end{figure}

Intuitively, low values for $M_h$ become asymptotically the larger $h$, as more bytes are contributing to the maximum value. We illustrate this in \cref{fig:ae_pmf}. 
Further, $\lim_{h\to\infty} E(M_h) = 255$.
For instance, with $h=2000$, $\mathrm{P}(M_h=255)>0.999$.
\cf~\eqref{eq:eight}).
That is, $\mathrm{P}(M_h=m\mid M_h\geq x)\geq\mathrm{P}(M_h=m)$ for any $0\leq x\leq 255$.

The practical implication of this is that when AE is used with target chunk sizes beyond \qty{2}{KB},
the approximation that $M_h\approx 255$ can be used to simplify the problem to

\begin{equation}
    \mathrm{P}(i+h\text{ is cut-point}) = \mathrm{P}(B_i=255) = \frac{1}{256}.
\end{equation}

On average, therefore, a chunk cut-point will be found after the evaluation of 256 bytes.
Hence, target chunk size for AE is $\mu\approx h+256$ for large values of $h$;
the parameterization is determined by $h\approx\mu-256$.
We continue with extended calculations for small target chunk sizes.

The probability for a random byte to fail the matching condition is

\begin{equation}
    \mathrm{P}(X < \max\{B_i\}_{i=1}^{h}) = \sum_{m=0}^{255} \mathrm{P}(X < m)\cdot\mathrm{P}(\max\{B_i\}_{i=1}^{h}=m).
\end{equation}

The probability in this form would apply to the first byte of the sequence, \ie, it is equivalent to $\mathrm{P}(B_1<\max\{B_i\}_{i=2}^{h+2})$.

The second byte $B_2$, which only gets evaluated under the pre-condition that $B_1<\max\{B_i\}_{i=2}^{h+1}$, faces the same condition as its precursor, but has a different probability as it is conditioned:

\begin{equation}
\begin{split}
    \mathrm{P}(B_2<\max\{B_i\}_{i=3}^{h+2}\mid B_1<\max\{B_i\}_{i=2}^{h+1})\\
    =\sum_{x=0}^{255} \mathrm{P}(B_2=x\mid B_1<\max\{B_i\}_{i=2}^{h+1})\cdot\mathrm{P}(x<\max\{B_i\}_{i=3}^{h+2}\mid B_1<\max\{B_i\}_{i=2}^{h+1})\\
    =\sum_{x=0}^{255} \Bigg( \mathrm{P}(B_2=x\mid B_1<\max\{B_i\}_{i=2}^{h+1}) \cdot
 \sum_{m=x+1}^{255} \mathrm{P}(\max\{B_i\}_{i=3}^{h+2}=m\mid B_1<\max\{B_i\}_{i=2}^{h+1}) \Bigg)
\end{split}
\label{eq:seven}
\end{equation}

The expectation of $B_2$ and the expectation of $\max\{B_i\}_{i=3}^{h+2}$ are shifted towards higher values, given that $B_1<\max\{B_i\}_{i=2}^{h+1}$.

The two conditional probabilities needed to solve \eqref{eq:seven} are less trivial. 
We are deriving $\mathrm{P}(B_2=x\mid B_1<\max\{B_i\}_{i=2}^{h+1})$ using Bayes' formula, which transforms the expression to

\begin{equation}
    \mathrm{P}(B_2=x\mid B_1<\max\{B_i\}_{i=2}^{h+1}) = \frac{\mathrm{P}(B_1<\max\{B_i\}_{i=2}^{h+1}\mid B_2=x)\cdot\mathrm{P}(B_2=x)}{\mathrm{P}(B_1<\max\{B_i\}_{i=2}^{h+1})}.
\end{equation}

We derive the inversed conditional probability $\mathrm{P}(B_1<\max\{B_i\}_{i=2}^{h+1}\mid B_2=x)$ in the following lemma.

\begin{lemma}
The probability of a byte $B_1$ being smaller than the maximum value among the $h$ bytes in its horizon, given that one of the bytes $B_2$ is known, can be expressed as

	\begin{equation}
	\begin{split}
    	\mathrm{P}(B_1 < \max\{B_i\}_{i=2}^{h+1})\mid B_2=x)=
	    \mathrm{P}(x\geq \max\{B_i\}_{i=3}^{h+1})\cdot\mathrm{P}(B_1<x) \;\oplus\;\\ 
 	   \mathrm{P}(\max\{B_i\}_{i=3}^{h+1}>x)\cdot\mathrm{P}(B_1<\max\{B_i\}_{i=3}^{h+1})\mid \max\{B_i\}_{i=3}^{h+1}>x)
	\end{split}
	\end{equation}
	\label{lemma:ae_prob1}
\end{lemma}

\begin{proof}
	Given $B_2=x$, we know that $\max\{B_i\}_{i=2}^{h+1}\geq x$. That is, either $x$ is the maximum in this horizon and $x\geq \max\{B_i\}_{i=3}^{h+1}$, or the remaining bytes are and $\max\{B_i\}_{i=3}^{h+1}>x$. 
\end{proof}

\begin{lemma}
	The probability distribution for the maximum value among $h$ bytes, given that the preceding byte is smaller than the maximum value in its horizon, 
	can be expressed as 
	\begin{equation}
	\begin{split}
    	\mathrm{P}(\max\{B_i\}_{i=3}^{h+2}=m\mid B_1<\max\{B_i\}_{i=2}^{h+1})
	    =(h-1)\cdot \mathrm{P}(B_3=m \land B_j\leq m\;\forall j\in[4,h+1] \mid B_1<\max\{B_i\}_{i=2}^{h+1}) \cdot \\ 
	    \mathrm{P}(B_{h+3}\leq m)+
    	\mathrm{P}(B_{h+3}=m)\cdot\mathrm{P}(B_3\leq m\mid B_1<\max\{B_i\}_{i=2}^{h+1})^{h-1}
	\end{split}
	\end{equation}
	\label{lemma:ae_prob}
\end{lemma}

\begin{proof}
%	We are describing the probability of any one byte $B_j\in \{B_i\}_{i=3}^{h+2}$ having the value $m$
%while all the remaining bytes $B_{k\neq j} \leq m$ in the horizon $k\in[3,h+2]$.
The expectation about a subset of bytes $\{B_i\}_{i=3}^{h+2} \cap \{B_i\}_{i=2}^{h+1} = \{B_i\}_{i=3}^{h+1}$ is influenced by the given condition,
\ie, all bytes in the target sequence except for its final byte $B_{h+2}$.
Intuitively, one byte will be $m$ while the remaining $h-1$ bytes of the intersecting horizon are $\leq m$.
By multiplying the chance for one of these bytes by $h-2$, we account for every byte in the intersecting horizon to be in place of the maximum value. 
In the formula, we used $B_3$ as an arbitrary placeholder, as any byte in the affected sequence yields identical chances.
Simultaneously, we also verify that the final (non-intersecting) byte $B_{h+3}\leq m$.
Finally, we account for the case that the final byte $B_{h+3}=m$ and all bytes in the conditioned sequence $\leq m$.
\end{proof}

We further derive the following probability in support of \cref{lemma:ae_prob}:
\begin{equation}
\begin{split}
  \mathrm{P}(B_3=m \land B_j\leq m\;\forall j\in[4,h+1] \mid B_1<\max\{B_i\}_{i=2}^{h+1}) \\ 
   	 = \mathrm{P}(B_3=m\mid B_1<\max\{B_i\}_{i=2}^{h+1})\cdot\mathrm{P}(B_4\leq m\mid B_1<\max\{B_i\}_{i=2}^{h+1})^{h-2}
\end{split}
\label{eq:ten}
\end{equation}

The evaluation of the expression in \eqref{eq:seven} using \cref{lemma:ae_prob1,lemma:ae_prob} 
accumulates six hierarchies of sum-loops. 
The complexity further depends on the size of $h$.
However, even with low values for $h$, 
the evaluation of the expression turned out to be computationally too expensive (we interrupted the execution after two hours).
Therefore, we deem exact analytical solutions impracticable.
We recommend an experimental approach for tuning $h$ for low target chunk sizes,
and making use of the approximation $h\approx\mu-256$ for target chunk sizes beyond \qty{2}{KB}.
