# Supplementary material for: A Thorough Investigation of Content-Defined Chunking Algorithms for Data Deduplication
Source: arXiv:2409.06066 source file (2024-09-28)
Supplement: Supplementary file 2 [file pci_stochastics.tex]

\begin{definition}
	In PCI, $i+w-1$ marks a cut-point if it is the first position for which $\sum_{j=i}^{i+w}\text{popcount}(B_j) \geq \theta$.
\end{definition}

The probability for a sequence of $w$ randomly distributed bytes $B_1,\ldots,B_w$ to accumulate a specific popcount $p$ is described as

\begin{equation}
	\mathrm{P}\left(\sum_{i=1}^w\text{popcount}(B_i)=p\right) = \frac{\binom{8w}{p}}{2^{8w}}.
\end{equation}

Therefore, we can trivially determine that for this byte sequence to match PCI's matching condition, the probability equals

\begin{equation}
	\mathrm{P}\left(\sum_{i=1}^w\text{popcount}(B_i)\geq\theta\right) = \sum_{p=\theta}^{2^{8w}} \frac{\binom{8w}{p}}{2^{8w}}.
	\label{eq:pci_p_first}
\end{equation}

For position $i+w$ to set a chunk boundary, all positions $j+w$ where $j<i$ must have subsequently failed the matching condition.

In \eqref{eq:pci_p_first}, we contemplate the probability for the first possible position in the byte sequence to mark a chunk boundary.
The next possible position (\ie, $1+w$) is contingent upon the preceding position failing to satisfy the matching condition. 
Additionally, the expectation regarding the popcount within its window is also influenced by this event.

Intuitively, $1+w$ sets a new chunk boundary only if the insufficiency of 1-bits in the preceding window is compensated for by the 1-bits introduced by the new byte, with the 1-bits of the leftmost byte that dropped out being deducted.
Formally, this is the event of $\text{popcount}(B_{w+1})-\text{popcount}(B_1) > \theta-\sum_{i=1}^w\text{popcount}(B_i)$.
This event occurs when the popcount in $B_1$ is $a\in[0,7]$,
the popcount in $B_2,\ldots,B_w$ is $m=[\theta-8, \theta-8+a]$,
and the popcount in $B_{w+1}$ is $z=[m, 8]$.
This probability is encapsulated in the following equation:

\begin{equation}
	\mathrm{P}\left(\sum_{i=2}^{w+1}\text{popcount}(B_i)\geq\theta \mid \sum_{i=1}^w\text{popcount}(B_i)<\theta\right) =
	\sum_{a=0}^7\left( \frac{\binom{8}{a}}{2^8} \cdot \sum_{m=a+1}^8 \left( \frac{\binom{w-8}{m}}{2^{w-8}} \cdot \sum_{z=m}^8 \frac{\binom{8}{z}}{2^8} \right) \right)
\end{equation}

As with AE and RAM (\cf \cref{app:ae_probs,app:ram_probs}),
the consideration for later chunk boundaries, \ie, $i=3,4,\ldots$, only increases the complexity of this equation as the events become recursively dependent on one another.
Because of the high complexity of this probability and the unavailability of an approximation, we recommend determining parameters in PCI empirically.
