# Supplementary material for: A Thorough Investigation of Content-Defined Chunking Algorithms for Data Deduplication
Source: arXiv:2409.06066 source file (2024-09-28)
Supplement: Supplementary file 3 [file ram_stochastics.tex]

\begin{definition}
	In RAM, $h+i$ marks a cut-point if it is the first position for which $B_i\geq\max\{B_{j>h}\}_{j=1}^{h}$.
\end{definition}

The case for RAM is more trivial than it is for AE.
As the maximum value $M_h=\max\{B_j\}_{j=0}$ is fixed, the expectation is not dependent on consecutive events. 

Based on the probability distribution about the maximum value among $h$ bytes we derived in \eqref{eq:ae_mh_m}, 
we can obtain its expected value through

\begin{equation}
	E(M_h)=\sum_{m=0}^{255} m\cdot\mathrm{P}(M_h=m).
\end{equation}

Here again, $\lim_{h\to\infty} E(M_h) = 255$.

The analysis of the relationship between $h$ and $\mu$ in RAM now breaks down to finding how many random bytes $X$ it takes \textit{on average} for one to be greater than or equal $M_h$:

\begin{equation}
\begin{aligned}
	&& x\cdot\mathrm{P}(X\geq E(M_h)) &= 1\\
	\Leftrightarrow && \qquad x&=\frac{1}{\mathrm{P}(X\geq E(M_h))}
\end{aligned}
\end{equation}

As $h$ acts as an inherent minimum chunk size, $\mu=h+x$, and therefore

\begin{equation}
	\mu = h + \frac{1}{\mathrm{P}(X\geq E(M_h))}.
\end{equation}

After insertion, we conclude the following formula in order to determine the target chunk size:

\begin{equation}
\begin{split}
	\mu &= h + \left(\frac{256
	-\sum_{m=0}^{255}m\cdot\left(\left(\frac{m+1}{256}\right)^h-\left(\frac{m}{256}\right)^h\right)}{256}\right)^{-1} \\
	&= h + \left(1-\frac{1}{256}\sum_{m=0}^{255}m\cdot\left(\left(\frac{m+1}{256}\right)^h-\left(\frac{m}{256}\right)^h\right)\right)^{-1} \\
	%	\mu &= h + \left(\frac{1}{256}-\frac{1}{256}\cdot\sum_{m=0}^{255} m \cdot \left( \left( \frac{m+1}{256} \right)^h - \left( \frac{m}{256} \right)^h \right) \right)^{-1} \\
%	\mu &= h + \left(256 - 256 \cdot \sum_{m=0}^{255} m \cdot \left( \left( \frac{m+1}{256} \right)^h - \left( \frac{m}{256} \right)^h \right) \right)^{-1} \\
%	\mu &= -h+ \frac{256}{\left(\frac{1}{256}\right)^h (256-\sum_{m=1}^{256} m\cdot((m+1)^h-m^h)}
\end{split}
\end{equation}

Because of its complex transcendental nature, we must solve $h$ numerically.

In addition to that, we can provide the same approximation for target chunk sizes beyond \qty{2}{KB} that we concluded in \cref{app:ae_probs}.
As $\lim_{h\to\infty}E(M_h)=255$, and $\mathrm{X\geq 255}=\frac{1}{256}$, we can akin to AE use the approximation $\mu\approx h+256$ for $h>$ \qty{2}{KB}.
